# Supplementary material for: Challenges in the use of quantum computing hardware-efficient Ansatze in electronic structure theory
Source: arXiv:2208.09832 ancillary file (2023-08-03)
Supplement: Supplementary file 1 [file si.pdf]

# Challenges in the use of quantum computing hardware-efficient Ansätze in electronic structure theory: Supplementary information

Ruhee D'Cunha and T. Daniel Crawford
*Department of Chemistry, Virginia Tech, Blacksburg, VA 24061, USA*

Mario Motta and Julia E. Rice
*IBM Quantum, IBM Research Almaden, 650 Harry Road, San Jose, CA 95120, USA*

## I. DETAILS OF THE DATABASE

The data presented in this study can be publicly accessed on GitHub at [1]. The schema is organized as shown in Figure S1.

Subfolders named "operators" contain files named mol_R_op.txt with the qubit representation of the operator $\mathsf{op} = \mathsf{h}, \mathsf{ne}, \mathsf{s2}, \mathsf{sz}, \mathsf{p}, \mathsf{php}$ (respectively Hamiltonian, electron number, total spin, spin-z, projector $\hat{\Pi}$ and product $\hat{\Pi}\hat{J}\hat{\Pi}$; the latter two operators are defined in Eq. (4) of the main text and employed in first-quantization calculations with padding scheme) for molecule mol at geometry $R$. Operators are stored in the format $(\mathsf{s}_1, c_1) \dots (\mathsf{s}_{n_P}, c_{n_P})$ where $\mathsf{s}_1 \dots \mathsf{s}_{n_P}$ are strings with entries $\mathsf{I}, \mathsf{X}, \mathsf{Y}, \mathsf{Z}$ for Pauli operators, and $c_1 \dots c_{n_P}$ are real-valued coefficients.

Subfolders named "circuits" contain files named mol_R_circuit.txt with the quantum circuits executed in this study. Circuits are stored in the format $(n_1, d_1, p_1) \dots (n_{n_g}, d_{n_g}, p_{n_g})$ where $n_k$ is the name of gate $k$, $d_k$ its domain (i.e. the qubits it acts upon) and $p_k$ any parameters labeling it (i.e. single-qubit rotation angles).

Operators and circuits are in plain text format, and can be read and processed with the Python scripts under auxiliary_material/scripts.

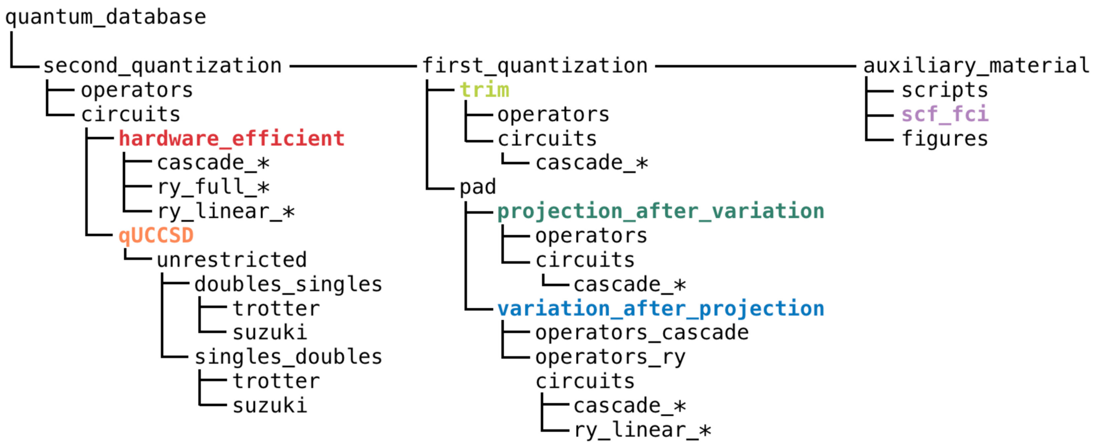


Figure S 1: Organization of the database accompanying this study. Data under hardware_efficient (red), qUCCSD (orange), trim (light green), projection_after_variation (dark green), variation_after_projection (blue) and scf_fci (purple) were used to generate figures in the main text and SI.

## II. CLASSICAL PREPROCESSING

The molecular geometries studied in this work are

- LiH: $\mathbf{R}_{\rm Li} = (0, 0, 0)$, $\mathbf{R}_{\rm H} = (0, 0, R)$ with $R = 0.7 + 0.1\ k$, $k = 0 \dots 28$
- BH: $\mathbf{R}_{\rm B} = (0, 0, 0)$, $\mathbf{R}_{\rm H} = (0, 0, R)$ with $R = 0.7 + 0.1\ k$, $k = 0 \dots 28$
- HF: $\mathbf{R}_{\rm F} = (0, 0, 0)$, $\mathbf{R}_{\rm H} = (0, 0, R)$ with $R = 0.7 + 0.1\ k$, $k = 0 \dots 38$
- $BeH_2$: $\mathbf{R}_{\rm Be} = (0, 0, 0)$, $\mathbf{R}_{\rm H_1} = (0, 0, -R)$; $\mathbf{R}_{\rm H_2} = (0, 0, R)$ with $R = 0.7 + 0.1\ k$, $k = 0 \dots 38$
- $H_2O$: $\mathbf{R}_{\rm O} = (0, 0, 0)$, $\mathbf{R}_{\rm H_1} = (R, 0, 0)$; $\mathbf{R}_{\rm H_2} = (R\cos(\theta), R\sin(\theta), 0)$ with $\theta = 104.4^o$, $R = 0.7 + 0.1\ k$, $k = 0 \dots 26$

For each selected molecule and geometry, we performed a second-order RHF calculation with molecular point-group symmetries, using PySCF [2, 3]. Convergence of energies and molecular orbitals was ensured, as well as stability of the RHF state under orbital rotations [4–8] and smoothness of the Fock operator eigenvalues as a function of $R$, as seen in the left portion of Figure S2. For each molecule and geometry, a FCI calculation was subsequently carried out, and the one-body density matrix was diagonalized to obtain occupation numbers, shown in the right portion of Figure S2.

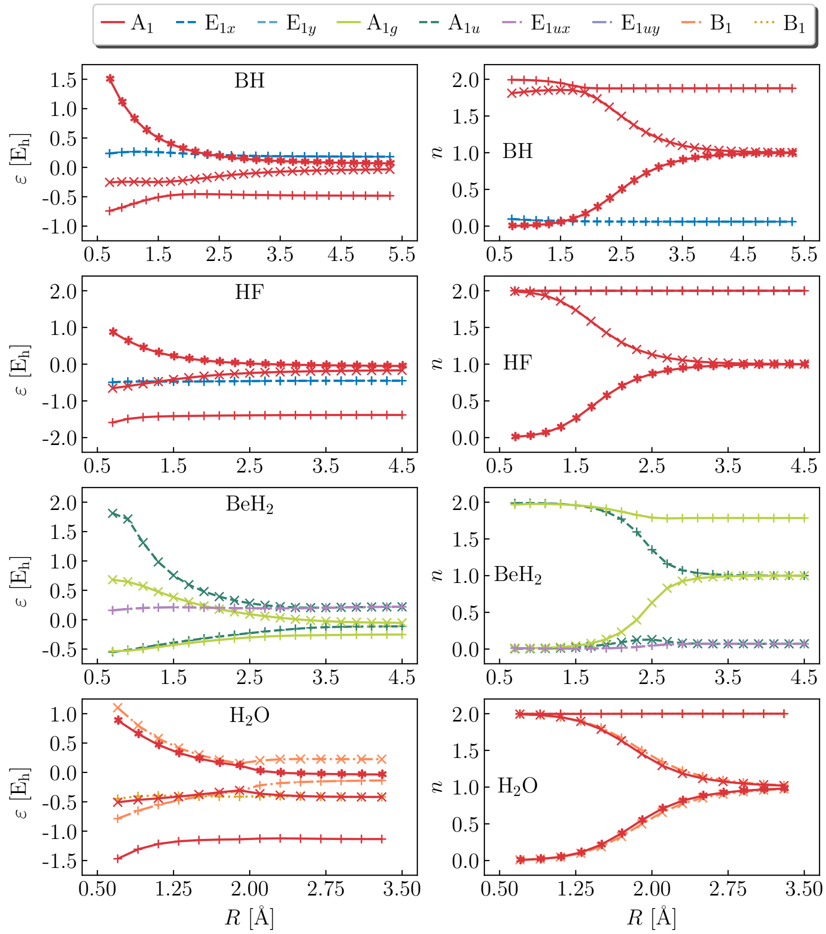


Figure S2: Eigenvalues of the Fock operator in Hartree units (left, $\varepsilon$) and occupation numbers of the exact ground-state one-body density matrix (right, $n$) for BH, HF, $BeH_2$ and $H_2O$ (top to bottom). Colors denote irreps of the molecular point-group symmetry; plus, cross, and asterisk markers denote orbitals in ascending order of energy within a specific irrep; the energy and occupation number of the core 1s orbital are omitted.

## III. Q-UCCSD

The development and characterization of unitary coupled-cluster Ansätze is a conceptually interesting and practically useful research area, at the interface between quantum computation and electronic structure.

Quantum computing literature has mostly focused on the quantum unitary coupled-cluster with singles and doubles (q-UCCSD). The performance of such an Ansatz (measured in both accuracy, computational cost, and symmetry breaking properties) is affected by implementation details, requiring a careful assessment. Some of these details are

1. the choice of a spin-unrestricted versus a spin-restricted cluster operator, respectively Eq. (8) and Eq. (9), (10) of the main text

2. the approximations used to implement the exponential Ansatz Eq. (7) of the main text; these include $(a)$ the chosen product formula, e.g. primitive Trotter or second-order Suzuki [9–12] $(b)$ the number of steps in the product formula $(c)$ the order in which exponentials of single- and double-excitation operators are composed within the chosen product formula

In the present work, we explored the effect of such implementation aspects on the q-UCCSD results for $H_2O$.

*a. Unrestricted and restricted closed-shell implementation.* The first step in the implementation of q-UCCSD is to write the cluster operator as

$$\hat{T} = \sum_{\mu=1}^{k} t_\mu \hat{O}_\mu \tag{1}$$

for suitable fermionic operators $\hat{O}_\mu$. In an unrestricted implementation of q-UCCSD, one simply has

$$\begin{aligned} \hat{T} &= \sum_{ai\sigma} t_{i\sigma}^{a\sigma} \hat{E}_{i\sigma}^{a\sigma} + \sum_{aibj\sigma\tau} t_{i\sigma,j\tau}^{a\sigma,b\tau} \hat{E}_{i\sigma,j\tau}^{a\sigma,b\tau} \,, \\ \hat{E}_{l_1\sigma_1,\dots,l_n\sigma_n}^{k_1\sigma_1,\dots,k_n\sigma_n} &= \hat{c}_{k_1\sigma_1}^\dagger \dots \hat{c}_{k_n\sigma_n}^\dagger \hat{c}_{l_n\sigma_n} \dots \hat{c}_{l_1\sigma_1} \,, \end{aligned} \tag{2}$$

where the factor 1/4 in Eq. (8) of the main text was dropped to avoid clutter. In a closed-shell implementation, the q-UCCSD operator is written as

$$\begin{aligned} \hat{T} &= \sum_{ai} t_i^a \Big( \sum_\sigma \hat{E}_{i\sigma}^{a\sigma} \Big) + \sum_{(ai)\le(bj)} \tilde{t}_{ij}^{ab} \Big( \sum_{\sigma\tau} \hat{E}_{[i\sigma,j\tau]}^{[a\sigma,b\tau]} \Big) \\ &= \sum_{ai} t_i^a \Big( \sum_\sigma \hat{E}_{i\sigma}^{a\sigma} \Big) + \sum_{ai} \tilde{t}_{ii}^{aa} \Big( 8\hat{E}_{i\alpha,i\beta}^{a\alpha,a\beta} \Big) + \sum_{a,i<j} \tilde{t}_{ij}^{aa} \Big( 4\hat{E}_{i\alpha,j\beta}^{a\alpha,a\beta} + 4\hat{E}_{j\alpha,i\beta}^{a\alpha,a\beta} \Big) + \sum_{a<b,i} \tilde{t}_{ii}^{ab} \Big( 4\hat{E}_{i\alpha,i\beta}^{a\alpha,b\beta} + 4\hat{E}_{i\alpha,i\beta}^{b\alpha,a\beta} \Big) \\ &+ \sum_{a<b,i<j} \tilde{t}_{ij}^{ab} \Big( \sum_\sigma \hat{E}_{i\sigma,j\sigma}^{a\sigma,b\sigma} - \hat{E}_{j\sigma,i\sigma}^{a\sigma,b\sigma} - \hat{E}_{i\sigma,j\sigma}^{b\sigma,a\sigma} + \hat{E}_{j\sigma,i\sigma}^{b\sigma,a\sigma} + 4\hat{E}_{i\alpha,j\beta}^{a\alpha,b\beta} + 4\hat{E}_{j\alpha,i\beta}^{b\alpha,a\beta} \Big) \\ &+ \sum_{a<b,i>j} \tilde{t}_{ij}^{ab} \Big( \sum_\sigma \hat{E}_{i\sigma,j\sigma}^{a\sigma,b\sigma} - \hat{E}_{j\sigma,i\sigma}^{a\sigma,b\sigma} - \hat{E}_{i\sigma,j\sigma}^{b\sigma,a\sigma} + \hat{E}_{j\sigma,i\sigma}^{b\sigma,a\sigma} + 4\hat{E}_{i\alpha,j\beta}^{a\alpha,b\beta} + 4\hat{E}_{j\alpha,i\beta}^{b\alpha,a\beta} \Big) \end{aligned} \tag{3}$$

where in the first passage we used a double antisymmetrization operator $X_{[c,d]}^{[a,b]} = X_{cd}^{ab} - X_{cd}^{ba} - X_{dc}^{ab} + X_{dc}^{ba}$ and in the second passage we observed that $(ai) \le (bj)$ indicates quartets of the form $a = b, i = j$, $a = b, i < j$, $a < b, i = j$, $a < b, i < j$, and $a < b, i > j$. Unlike in the unrestricted implementation, the operators

$$\hat{O}_i^a = \sum_\sigma \hat{E}_{i\sigma}^{a\sigma} \quad , \quad \hat{O}_{ij}^{ab} = \sum_{\sigma\tau} \hat{E}_{[i\sigma,j\tau]}^{[a\sigma,b\tau]} \tag{4}$$

commute with the total spin operator.

*b. Approximate exponential.* Having written the anti-hermitian cluster operator in the form $\hat{T} - \hat{T}^\dagger = \sum_{\mu=1}^k t_\mu (\hat{O}_\mu - \hat{O}_\mu^\dagger)$, its exponential is written as a product of $n_l$ identical terms,

$$e^{\hat{T}-\hat{T}^\dagger} = \left( e^{\frac{\hat{T}-\hat{T}^\dagger}{n_l}} \right)^{n_l} \quad , \tag{5}$$

and each term is approximated with a product formula. In this work, we compared the primitive Trotter and second-order Suzuki formulas,

$$\begin{aligned} e^{\frac{\hat{T}-\hat{T}^\dagger}{n_l}} &\to e^{\frac{t_k(\hat{O}_k-\hat{O}_k^\dagger)}{n_l}} \dots e^{\frac{t_1(\hat{O}_1-\hat{O}_1^\dagger)}{n_l}} \text{ (Trotter)} \\ e^{\frac{\hat{T}-\hat{T}^\dagger}{n_l}} &\to e^{\frac{t_1(\hat{O}_1-\hat{O}_1^\dagger)}{2n_l}} \dots e^{\frac{t_k(\hat{O}_k-\hat{O}_k^\dagger)}{n_l}} \dots e^{\frac{t_1(\hat{O}_1-\hat{O}_1^\dagger)}{2n_l}} \text{ (Suzuki)} \end{aligned} \tag{6}$$

It should be noted that the order of operators affects the results of a simulation. In this work, we compared an implementation where singles are followed by doubles and one where doubles are followed by singles.

Finally, each operator $\hat{O}_\mu - \hat{O}_\mu^\dagger$ is mapped, exactly as in the case of other operators (e.g. the Hamiltonian and particle number operators) onto a qubit operator, i.e. a linear combination of Pauli operators, $\hat{O}_\mu - \hat{O}_\mu^\dagger = \sum_i c_{i\mu} \, \sigma_{\mathbf{v}_i \mathbf{w}_i}$, and the exponential of such an operator is mapped onto the quantum circuit

$$e^{\frac{t_\mu(\hat{O}_\mu-\hat{O}_\mu^\dagger)}{2n_l}} \to \prod_i e^{\frac{t_\mu c_{i\mu}}{2n_l} \sigma_{\mathbf{v}_i \mathbf{w}_i}} \, . \tag{7}$$

It should be noted that, unless the operators $\sigma_{\mathbf{v}_i \mathbf{w}_i}$ commute with each other, an additional primitive Trotter approximation is introduced in the passage from fermionic operators to quantum circuits. In a closed-shell implementation, such an approximation in general leads to breaking of the spin symmetry, since the left member of Eq. (7) commutes with the total spin operator, but its qubit representation in general does not.

The quantum circuits corresponding to Eq. (7) are well-known in Jordan-Wigner representation [13], where they take the form shown in Figure S3.

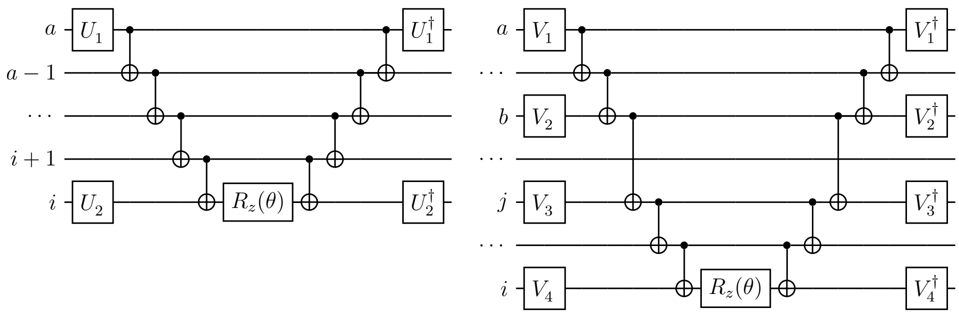


Figure S 3: Quantum circuits for the exponentiation of the single (left) and double (right) excitation operators in the q-UCCSD Ansatz in a Jordan-Wigner representation. Indices $a, b, i, j$ label occupied and virtual spin-orbitals, and Clifford unitaries are $(U_1, U_2) = \{(A_Y, A_X), (A_X, A_Y)\}$ for singles, and $(V_1, V_2, V_3, V_4) = (A_X, A_X, A_Y, A_X)$, $(A_Y, A_X, A_Y, A_Y)$, $(A_X, A_Y, A_Y, A_Y)$, $(A_X, A_X, A_X, A_Y)$, $(A_Y, A_X, A_X, A_X)$, $(A_X, A_Y, A_X, A_X)$, $(A_Y, A_Y, A_Y, A_X)$, $(A_Y, A_Y, A_X, A_Y)\}$ for doubles, with $A_X = H$ and $A_Y = HS$ and $H$, $S$ denoting the Hadamard and $S$ gates respectively.

## IV. ADDITIONAL FIRST-QUANTIZATION SIMULATIONS

In Figure 4 we compute the ground-state potential energy curves for the BH, HF, $BeH_2$, and $H_2O$ molecules (left to right), using the "trimming" scheme. In Figures 5 and 6 we use instead the "padding" scheme, detailed in the Appendix, where $K \leq 2^{n_q}$. These figures illustrate the cascade and linear-connectivity $R_y$ Ansätze with the variation-after-projection optimization.

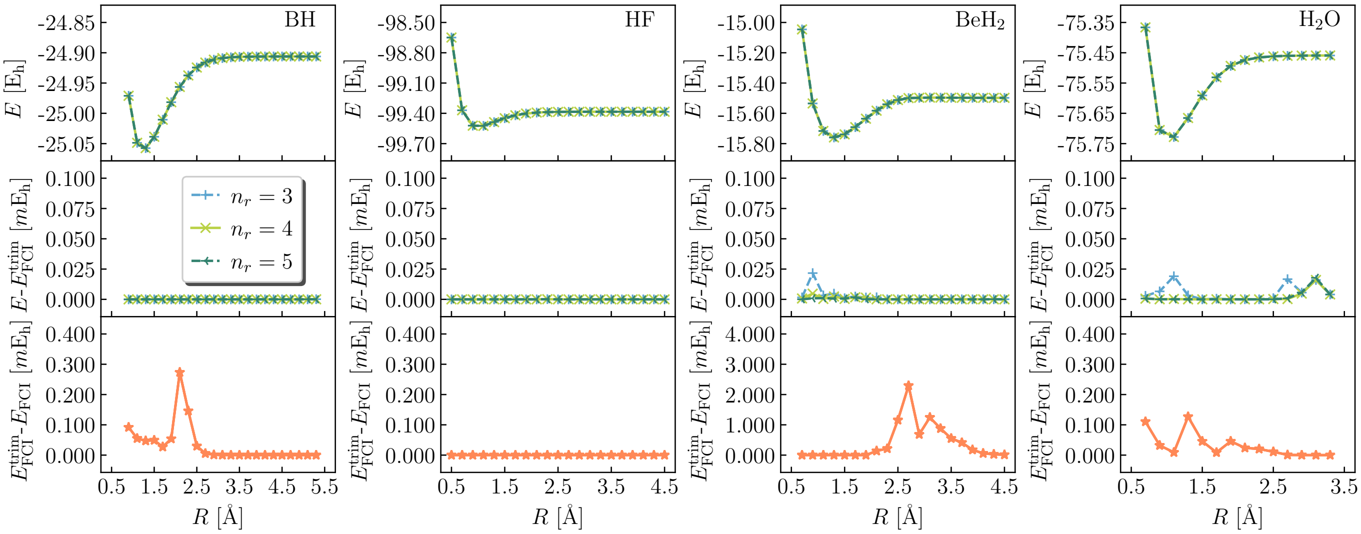


Figure S4: Total energy, deviation between computed and exact total energy using a first-quantization encoding and a trimming procedure for qubit reduction, and energy error from the trimming procedure (top to bottom) for the BH, HF, $BeH_2$ and $H_2O$ molecules at the STO-6G level (left to right) using the cascade Ansatz.

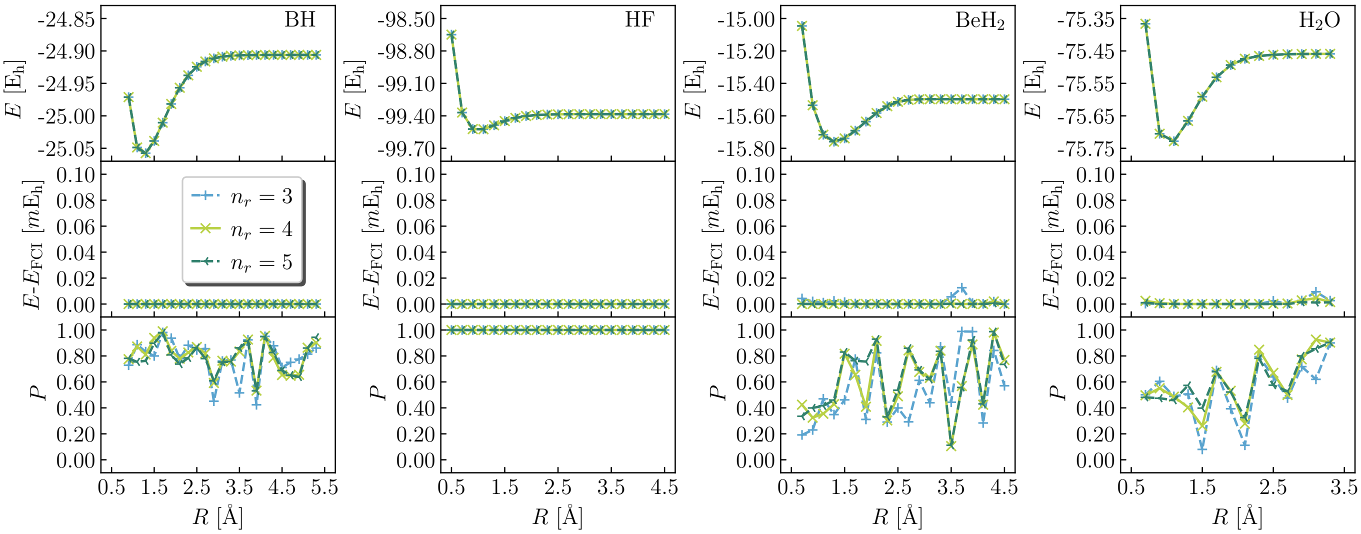


Figure S5: Total energy, deviation between computed and exact energy, and squared-norm of the physical component of the wavefunction (top to bottom) for the BH, HF, $BeH_2$ and $H_2O$ molecules at the STO-6G level (left to right) using a first-quantization encoding with padding and a cascade Ansatz optimized with the variation-after-projection scheme.

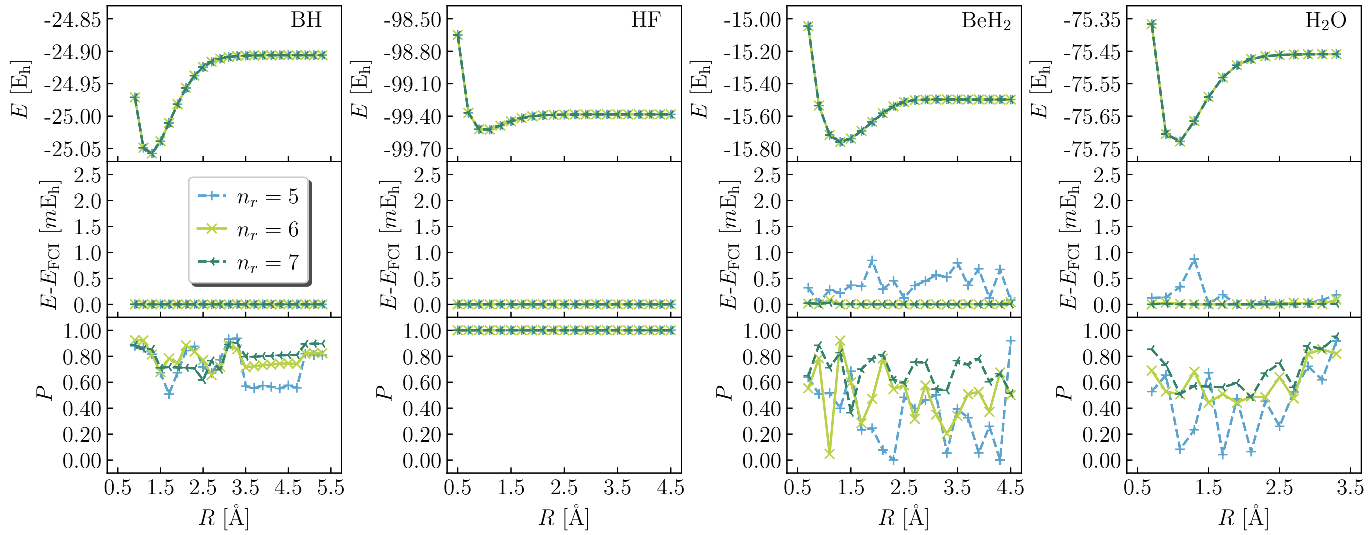


Figure S6: Total energy, deviation between computed and exact energy, and squared-norm of the physical component of the wavefunction (top to bottom) for the BH, HF, $BeH_2$ and $H_2O$ molecules at the STO-6G level (left to right) using a first-quantization encoding with padding and an $R_y$ Ansatz with linear connectivity optimized with the variation-after-projection scheme.

# V. ADDITIONAL SECOND-QUANTIZATION CALCULATIONS

In this Section, we illustrate additional second-quantization calculations. For each molecule, we report total energies and deviations between computed and exact total energies in a figure, and deviations between computed and exact total particle number, spin-$z$ and total spin in a second figure. In a dedicated Subsection, we illustrate calculations for LiH employing second quantization and the standard Jordan-Wigner mapping without qubit tapering.

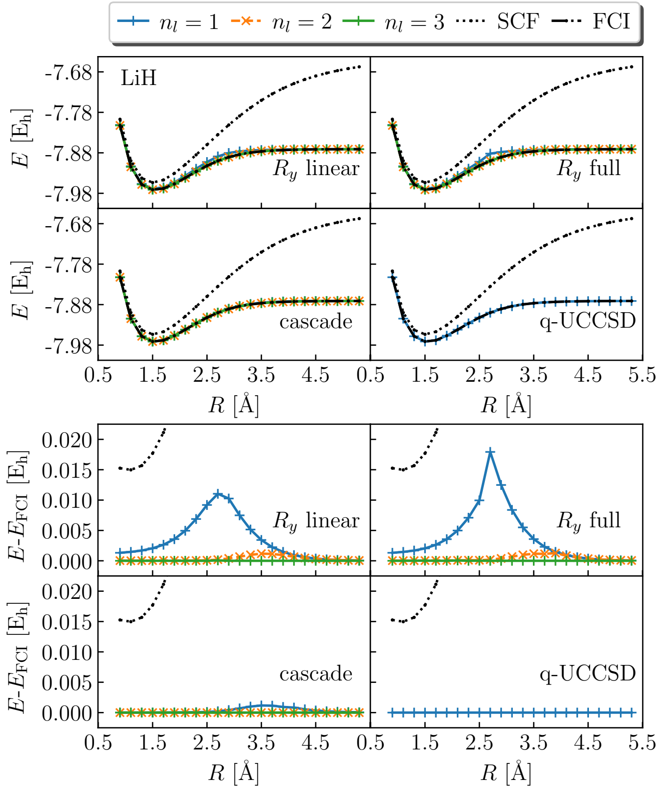


Figure S7: Total energy (top chart) and deviation between computed and exact total energy (bottom chart) using the $R_y$ (with linear- and full-connectivity), cascade, and q-UCCSD Ansätze (left to right), for the LiH molecule at the STO-6G level.

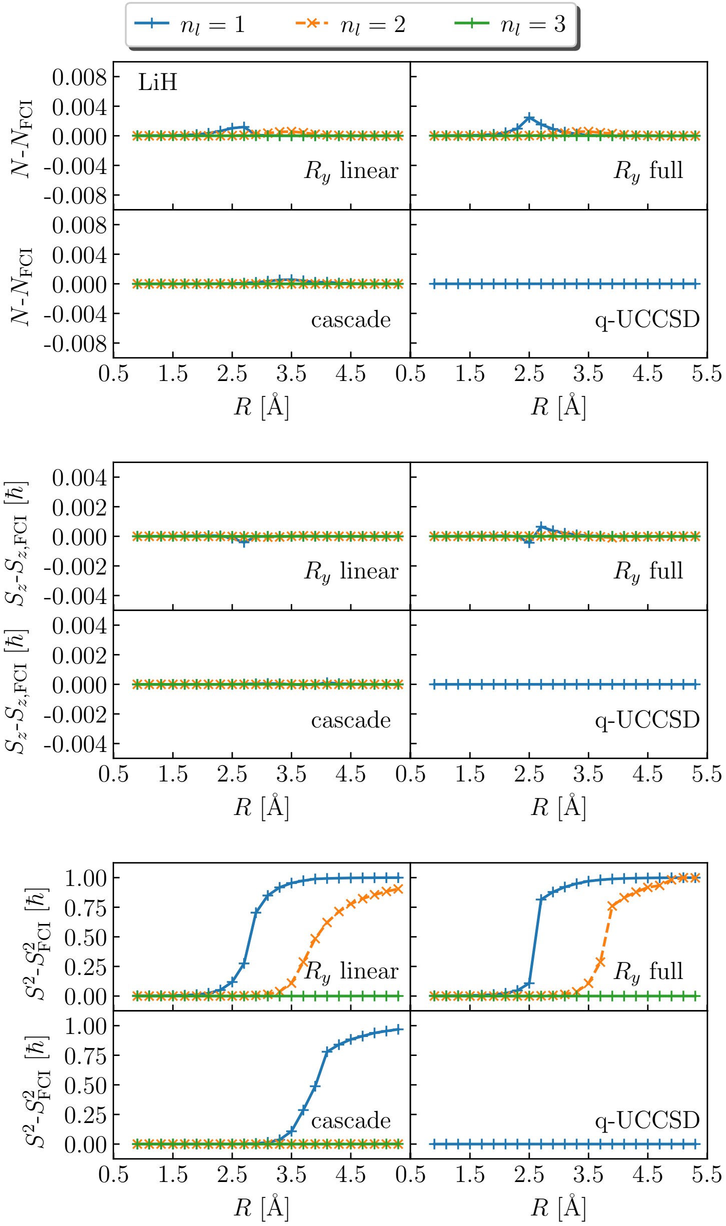


Figure S8: Deviation between computed and exact electron number, total spin, and spin-$z$ (top to bottom) using the $R_y$ (with linear- and full-connectivity), cascade, and q-UCCSD Ansätze (left to right), for the LiH molecule at the STO-6G level.

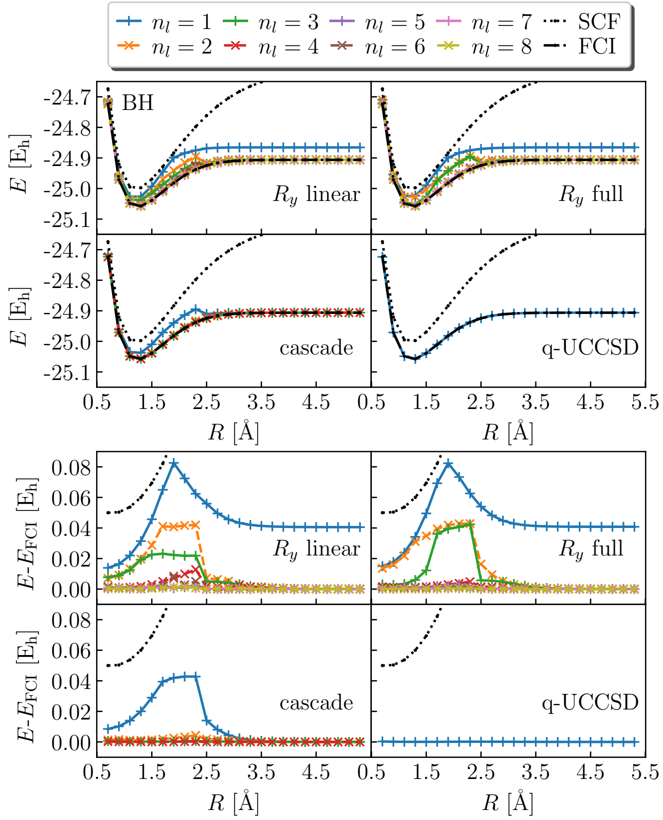


Figure S9: Total energy (top chart) and deviation between computed and exact total energy (bottom chart) using the $R_y$ (with linear- and full-connectivity), cascade, and q-UCCSD Ansätze (left to right), for the BH molecule at the STO-6G level.

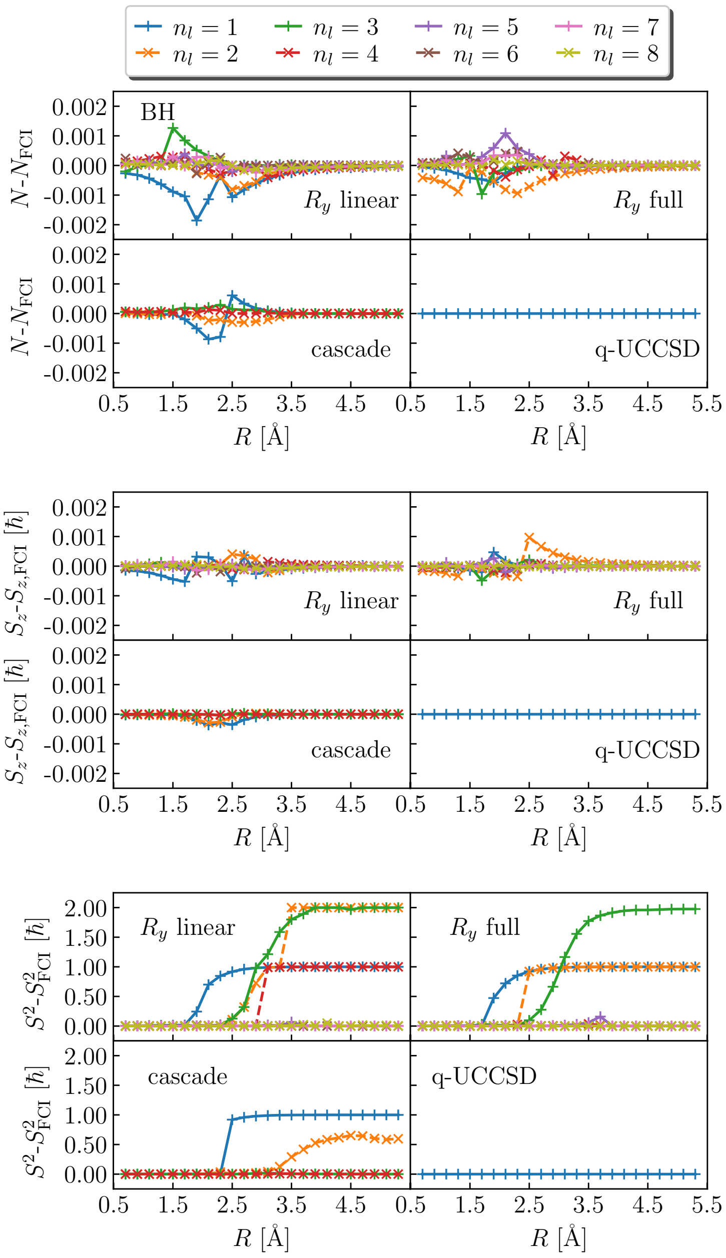


Figure S10: Deviation between computed and exact electron number, total spin, and spin-$z$ (top to bottom) using the $\mathrm{R}_y$ (with linear- and full-connectivity), cascade, and q-UCCSD Ansätze (left to right), for the BH molecule at the STO-6G level.

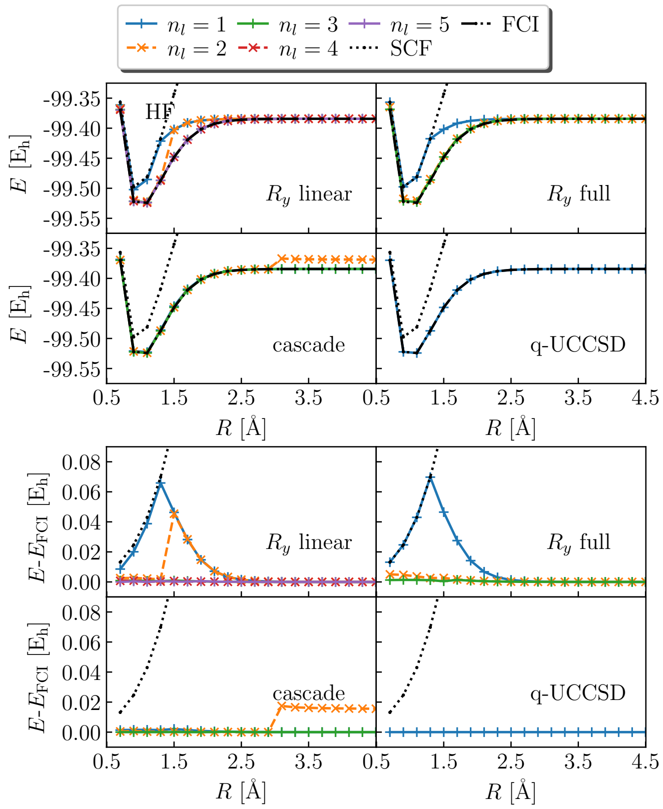


Figure S11: Total energy (top chart) and deviation between computed and exact total energy (bottom chart) using the $R_y$ (with linear- and full-connectivity), cascade, and q-UCCSD Ansätze (left to right), for the HF molecule at the STO-6G level.

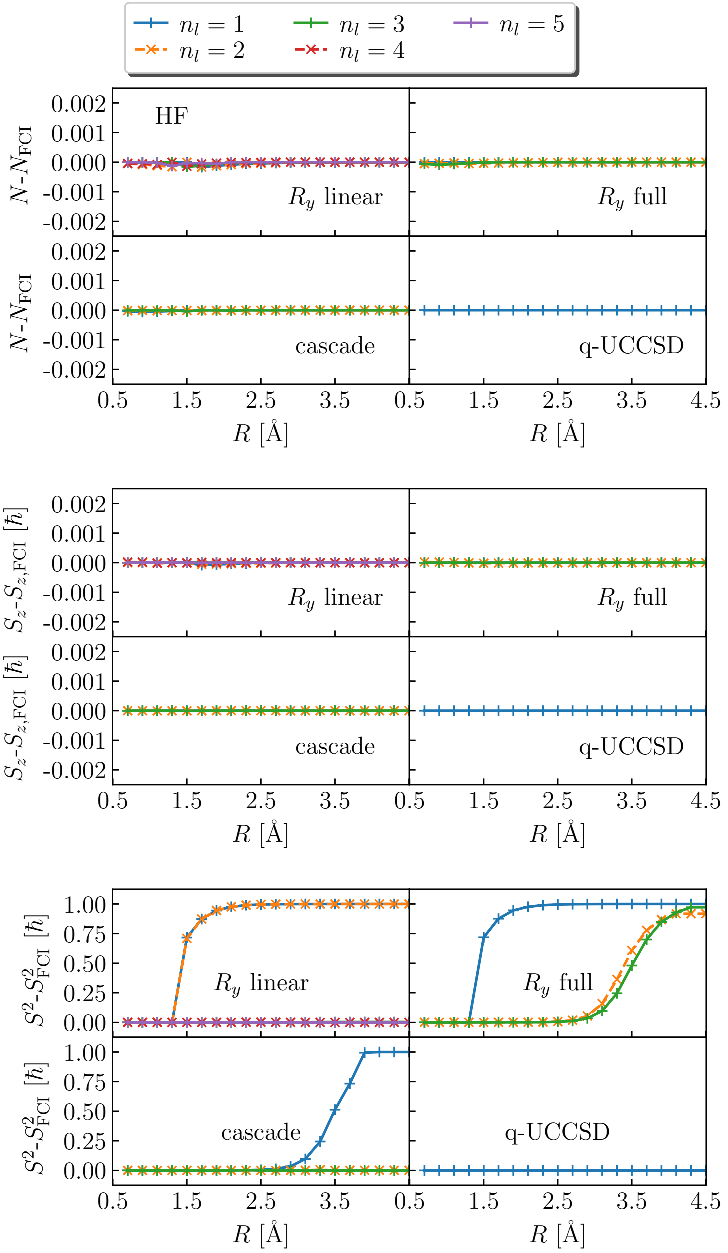


Figure S12: Deviation between computed and exact electron number, total spin, and spin-$z$ (top to bottom) using the $R_y$ (with linear- and full-connectivity), cascade, and q-UCCSD Ansätze (left to right), for the HF molecule at the STO-6G level.

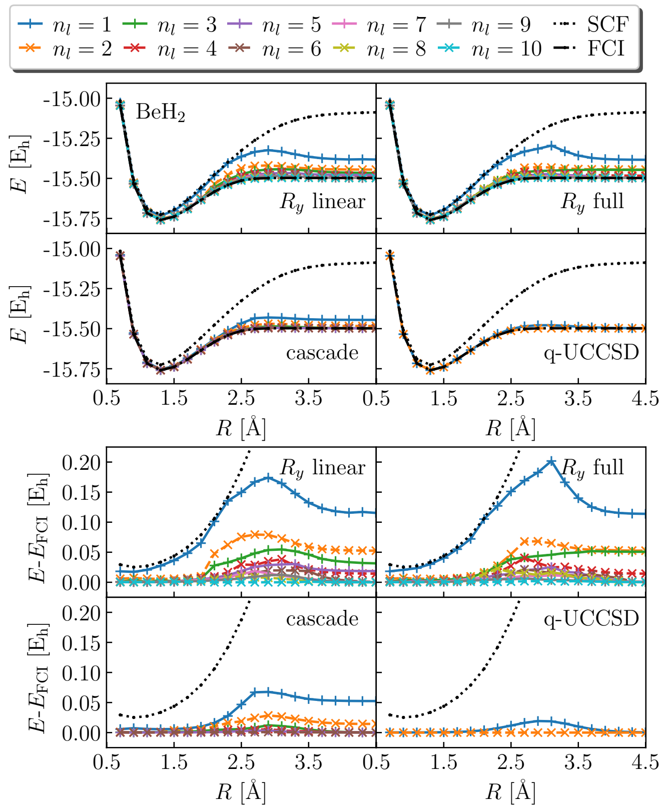


Figure S13: Total energy (top chart) and deviation between computed and exact total energy (bottom chart) using the R$_y$ (with linear- and full-connectivity), cascade, and q-UCCSD Ansätze (left to right), for the BeH$_2$ molecule at the STO-6G level.

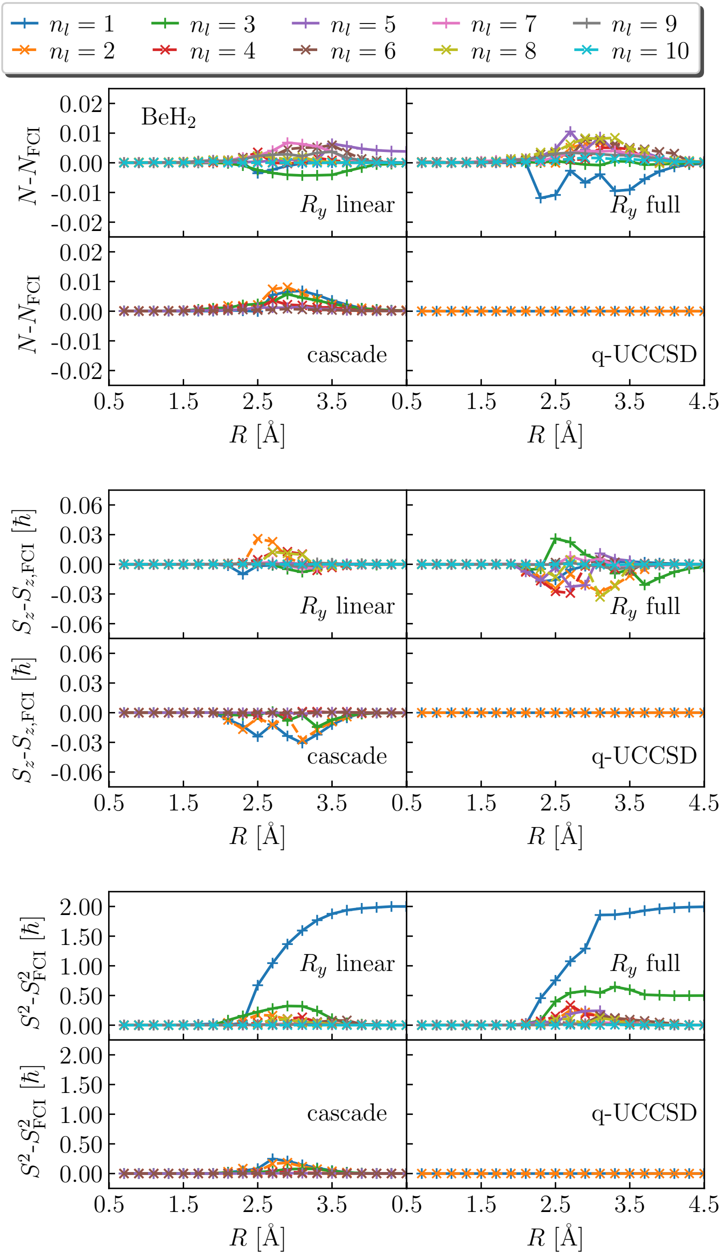


Figure S14: Deviation between computed and exact electron number, total spin, and spin-$z$ (top to bottom) using the $R_y$ (with linear- and full-connectivity), cascade, and q-UCCSD Ansätze (left to right), for the $BeH_2$ molecule at the STO-6G level.

### A. Calculations in Jordan-Wigner representation

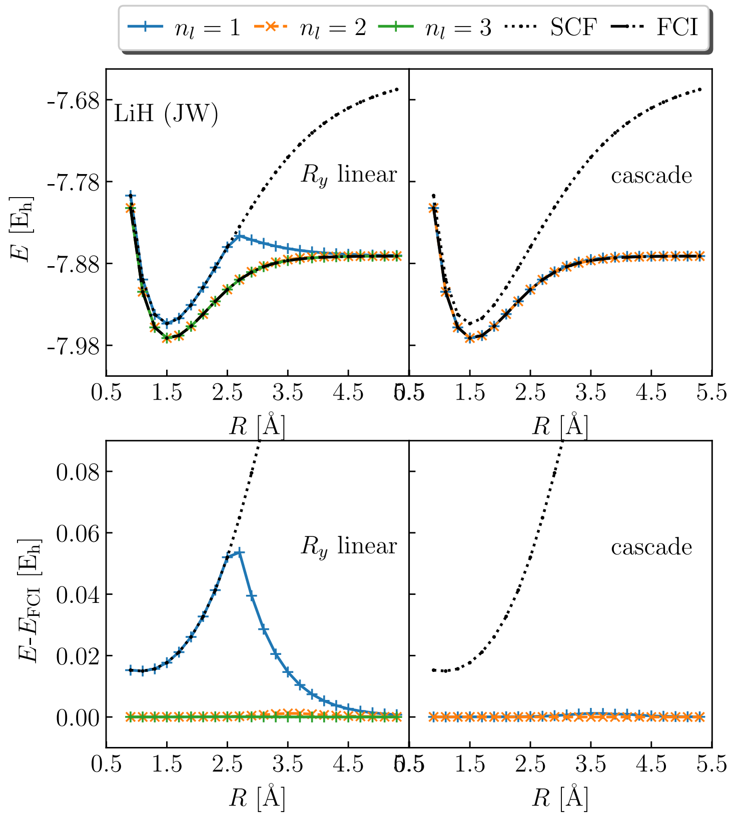


Figure S15: Total energy (top chart) and deviation between computed and exact total energy (bottom chart) using the $R_y$ (with linear- and full-connectivity), cascade, and q-UCCSD Ansätze (left to right), for the LiH molecule at the STO-6G level. We employ the Jordan-Wigner second quantization representation.

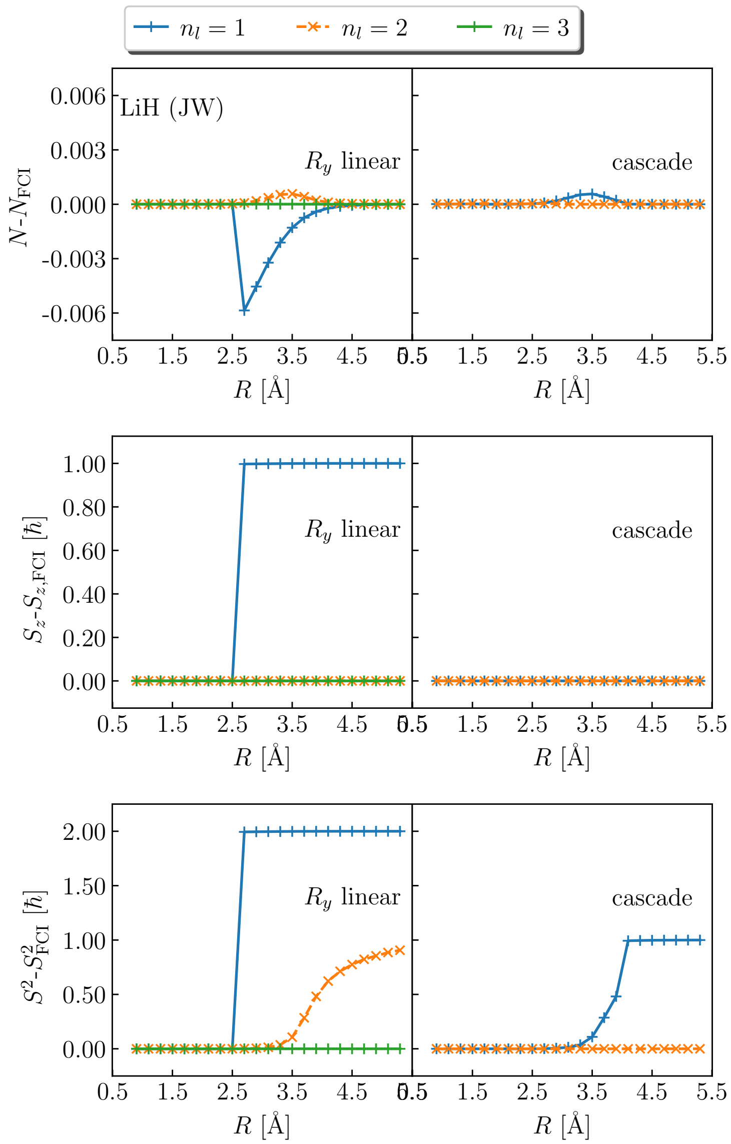


Figure S16: Deviation between computed and exact electron number, total spin, and spin-$z$ (top to bottom) using the $R_y$ (with linear- and full-connectivity), cascade, and q-UCCSD Ansätze (left to right), for the LiH molecule at the STO-6G level. We employ the Jordan-Wigner second quantization representation.

[1] R. D'Cunha, T. D. Crawford, M. Motta, and J. E. Rice, https://github.com/mariomotta/quantum_database (2022).
[2] Q. Sun, T. C. Berkelbach, N. S. Blunt, G. H. Booth, S. Guo, Z. Li, J. Liu, J. D. McClain, E. R. Sayfutyarova, S. Sharma, *et al.*, WIREs Comput. Mol. Sci **8**, e1340 (2018).
[3] Q. Sun *et al.*, J. Chem. Phys **153**, 024109 (2020).
[4] J. Čížek and J. Paldus, J. Chem. Phys **47**, 3976 (1967).
[5] K. Deguchi, K. Nishikawa, and S. Aono, J. Chem. Phys **75**, 4165 (1981).
[6] W. D. Allen, D. A. Horner, R. L. Dekock, R. B. Remington, and H. F. Schaefer III, Chem. Phys **133**, 11 (1989).
[7] Y. Yamaguchi, I. L. Alberts, J. D. Goddard, and H. F. Schaefer III, Chem. Phys **147**, 309 (1990).
[8] N. A. Burton, Y. Yamaguchi, I. L. Alberts, and H. F. Schaefer III, J. Chem. Phys **95**, 7466 (1991).
[9] H. F. Trotter, Proc. AMS **10**, 545 (1959).
[10] M. Suzuki, J. Math. Phys **32**, 400 (1991).
[11] A. M. Childs, Y. Su, M. C. Tran, N. Wiebe, and S. Zhu, Phys. Rev. X **11**, 011020 (2021).
[12] M. Suzuki, Comm. Math. Phys **51**, 183 (1976).
[13] P. K. Barkoutsos, J. F. Gonthier, I. Sokolov, N. Moll, G. Salis, A. Fuhrer, M. Ganzhorn, D. J. Egger, M. Troyer, A. Mezzacapo, S. Filipp, and I. Tavernelli, Phys. Rev. A **98**, 022322 (2018).
